# Supplementary material for: FogMQ: A Message Broker System for Enabling Distributed, Internet-Scale IoT Applications over Heterogeneous Cloud Platforms
Source: arXiv:1610.00620 source file (2016-10-03)
Supplement: Supplementary file 1 [file appendix.tex]

We now prove Theorem\ref{theorem1}
\begin{proof}

    Let $\sigma^{t}$ and $w_x^{t}$ denote the game outcome and the weight of $x$ at round $t$ respectively, and let
    $\Delta w_x = w_x^{t+1} - w_x^{t}$.
        If $\migrate{i}{x}{y}$, then
        $$ u_i(y) f(w_y + u_i(y)) \leq  \eta  u_i(x) f(w_x - u_i(x)).$$
        As $ f \approx 1$,
        \begin{equation}
        \label{eq:state1}
          u_i(y) \leq \eta u_i(x).
        \end{equation}
        Because of the migration:
        $\Delta w_x < 0$ and
        $\Delta w_y > 0$,
        but $\left| \Delta w_x \right| \geq  u_i(x)$,
        and $\left| \Delta w_y \right| \leq  u_i(y).$ otherwise $i$ would not migrate, then
        \begin{equation}
        \label{eq:state2}
          \left| \Delta w_y \right| \leq \left| \Delta w_x \right| .
        \end{equation}
        Let $z_i=u_i(x_i) f(w_{x_i})$ denote the regularized weighted average latency and let $z_i^t$ denote its value at round $t$. After the migration, $i$'s peers split into two subsets:
        $V_{\text{inc}} = \{j \in V: z_j^{t+1} > z_j^{t} )\},$ and
        $V_{\text{dec}}= \{j \in V: z_j^{t+1} < z_j^{t} )\}.$
        Assume after the migration step that
        $\sum_{j \in V_{\text{inc}}} z_j  > \sum_{k \in V_{\text{dec}}} z_k.$
        Again for $f \approx 1$,
        $\sum_{j \in V_{\text{inc}}} u_j(x_j) > \sum_{k \in V_{\text{dec}}} u_k(x_k).$ Substitute with the weighted average latency value from \eqref{eq:latency} and since the demands (i.e. $d_{ij}$) remain unchanged,
        $\sum_{j \in V_{\text{inc}}} l(x_j, y) > \sum_{k \in V_{\text{dec}}} l(x_k, y).$
        By the reciprocity of $l$,
        $\sum_{j \in V_{\text{inc}}} l(y, x_j) > \sum_{k \in V_{\text{dec}}} l(y, x_k),$ and
        $u_i(y) \geq u_i(x)$, which contradicts \eqref{eq:state1}.
        By this contradiction and from \eqref{eq:state2}, the social value $C(\sigma^{t+1}) \leq C(\sigma^{t})$. Since $n$ and $m$ are finite and $C(\sigma) > 0$, then \protocol~must converge to a Nash equilibrium. $\blacksquare$
 \end{proof}

We now prove Lemma \ref{lemma1}

 \begin{proof} Let $\sigma$ denote a Nash outcome and $\sigma^*$ denote any alternative outcome. Also let $w_x$ and $w_x^*$ denote the weight on $x$ in outcomes $\sigma$  and $\sigma^*$ respectively. Similarly, let $x_i$ and $x_i^*$ denote $i$'s strategy (hosting cloud) in $\sigma$  and $\sigma^*$ respectively.
By definition of a Nash outcome, $\forall i,\; u_i(x_i) f(w_{x_i}) \leq u_i(x_i^*) f(w_{x_i^*}).$
Summing over all \acp{vm} we get,
$C(\sigma) = \sum_{i \in V} u_i(x_i) f(w_{x_i}) \leq \sum_{i \in V} u_i(x_i^*) f(w_{x_i^*})$
However,
\begin{equation*}
\begin{split}
\sum_{i \in V} u_i(x_i^*) f(w_{x_i^*}) &  \leq \sum_{x \in A}
\sum_{i: x_i = x} u_i(x) f(w_x + u_i(x) )  \\
 & \leq \sum_{x \in A}  w_x^* f(w_x + w_x^* ) \\
 & \leq \sum_{x \in A}  \lambda  w_x^* f(w_x^* ) + \varepsilon w_x f(w_x) \\
 &  = \lambda C(\sigma^*) + \varepsilon C(\sigma).
\end{split}
\end{equation*}
Then,  $C(\sigma) \leq \lambda C(\sigma^*) + \varepsilon C(\sigma).$
Rearranging we get,
$\text{POA} = C(\sigma)/C(\sigma^*) \leq \lambda / (1-\varepsilon).$
$\blacksquare$

\end{proof}
